# Supplementary material for: Plasmonically assisted channels of photoemission from metals
Source: arXiv:2105.01396 ancillary file (2021-05-04)
Supplement: Supplementary file 1 [file plas2PP_SM.pdf]

# SUPPLEMENTARY MATERIAL
# Plasmonically assisted channels of photoemission from metals

Dino Novko,[1] Vito Despoja,[1] Marcel Reutzel,[2] Andi Li,[3] Hrvoje Petek,[3] and Branko Gumhalter[1]
[1]*Institute of Physics, HR 10000 Zagreb, Croatia*
[2]*I. Physikalisches Institut, Georg-August-Universität Göttingen, D-37077 Göttingen, Germany*
[3]*Department of Physics and Astronomy and Pittsburgh Quantum Institute, University of Pittsburgh, Pittsburgh, Pennsylvania 15260, USA*

## S1. REGULARIZATION OF EXPRESSION (33)

The seemingly divergent expression (33) [1] which contains a square of $\delta$-function must be regularized before its application in expressions requiring the limits $t \to \infty$ and $t_x \to -\infty$. This procedure depends on the boundary conditions imposed on the wavefunctions solving the electronic Hamiltonian $H_0^{el}$ in Eq. (5). Here we shall distinguish two situations, **A.** the scattering boundary conditions, and **B.** the decaying states boundary conditions.

### A. Scattering boundary conditions

In this case the regularization depends on the normalization of electronic states appropriate to model description of electron yield across the surface in the sequential scenario of non-Einsteinian photoemission involving plasmons as monochromatic pump field for electron emission. This introduces a preferential coordinate, say $z$, with $z = 0$, $z < 0$ and $z > 0$ denoting the surface, the interior and the exterior of a semi-infinite system, respectively. To introduce convenient normalization of electron states we introduce the electron and plasmon quantum numbers and energy, respectively, using the notation $\mathbf{k} = (\mathbf{K}, k_z)$, $\mathbf{q} = (\mathbf{Q}, q_z)$ and $\epsilon_{\mathbf{k}} = \epsilon_{\mathbf{K}} + \epsilon_{k_z}$. In this case the $\delta$-function in expression (33) can be written in the form

$$2\pi\delta(\epsilon_{\mathbf{K}} + \epsilon_z - \epsilon_{\bar{\mathbf{K}}'} - \epsilon'_z \mp \hbar\omega_{\mathbf{q}}) \tag{S1}$$

with $\mp$ denoting the plasmon emission and absorption processes respectively. The primed quantities may also refer to a different band. To facilitate the derivations we retain the standard box normalization for the running waves whose propagation parallel to the surface is described by the quantum number $\mathbf{K}$, viz.

$$\langle \mathbf{K}|\mathbf{K}'\rangle = \delta_{\mathbf{K},\mathbf{K}'} = \left(\frac{2\pi}{L}\right)^2 \delta(\mathbf{K} - \mathbf{K}'), \tag{S2}$$

where again the band indices are implicit in $\delta_{\mathbf{K},\mathbf{K}'}$. Here $L$ is the quantization length in the directions parallel to the surface. To introduce normalization for the states describing electron propagation in the $z$-direction we follow the arguments leading to expressions (88)-(92) and (261)-(262) of Ref. [S1]. Two situations can be distinguished regarding the electron motion in the surface potential $V(z)$ with the property $V(z \to -\infty) < V(\to \infty) = E_V$ where $E_V$ is the vacum level energy, i.e. the cases $\epsilon_z < E_V$ and $\epsilon_z > E_V$.

*(i)* The states with $V(z \to -\infty) < \epsilon_z = \frac{\hbar^2 p_z^2}{2m} + V(-\infty) < E_V$, where $m$ is the electron mass, are nondegenerate stationary waves confined to the interior $z < 0$ (because of the total reflection at the surface). Their constituents, i.e. the incoming and outgoing waves, have the same asymptotic amplitudes which are taken to be unity. Here the wavevector $p_z = \sqrt{2m(\epsilon_z - V(-\infty))/\hbar^2}$ associated with either direction of motion in the region of large negative $z$ is a good quantum number. In this case the transition from box to continuum normalization reads

$$\langle p'_z|p_z\rangle = \delta_{p_z,p_z} = \frac{2\pi}{L_z}\delta(p'_z - p_z), \tag{S3}$$

where $L_z$ is the quantization length in the $z$-direction. Hence, the modulus of the currents associated with the incoming and outgoing components of the stationary wave $|p_z\rangle$ is

$$j_{p_z} = \frac{\hbar p_z}{m L_z} \tag{S4}$$

When both $\epsilon_z < E_V$ and $\epsilon'_z < E_V$ the energy conservation (S1) applied to plasmon emission or absorption in electron transitions between the states $|\mathbf{K}, p_z\rangle$ and $|\bar{\mathbf{K}}, p'_z\rangle$ yields

$$p'_z = \sqrt{2m(\epsilon_{\mathbf{K}} - \epsilon_{\bar{\mathbf{K}}} + \hbar^2 p_z^2/2m \mp \hbar\omega_{\mathbf{q}}})/\hbar. \tag{S5}$$

The corresponding currents are obtained from Eq. (S4).

*(ii)* Emission of an electron out of the sample can take place provided its asymptotic kinetic energy $\epsilon_z$ of the outward motion in the positive $z$-direction exceeds $E_V$. The states with $\epsilon_z > E_V$ are doubly degenerate. Each value of $\epsilon_z > E_V$ defines two linearly independent states[S5] which can be constructed so as to comprise two incoming waves approaching the surface from opposite directions and only one outgoing wave travelling away from

[1] Hereafter all numerals in round brackets that are not preceded by S refer to equations of the main text.

the surface either outward or inward. The states describing photoemission are those with only one outgoing wave which propagates from the surface to the right with unit amplitude and wavevector $k_z = \sqrt{2m(\epsilon_z - V(\infty))/\hbar^2}$. These are known as the inverse LEED states, hereafter indexed by $\mathcal{R}$ (right). Hence, the pair $(k_z, \mathcal{R})$ makes a good quantum number for description of the $z$-component of an inverse LEED state $|k_z, \mathcal{R}\rangle$. The corresponding degenerate counterpart is denoted by $|p_z, \mathcal{L}\rangle$. It describes the state with only one outgoing wave propagating from the surface to the left $z \to -\infty$ (index $\mathcal{L}$) with the wavevector $p_z$ and unit amplitude. The two asymptotic wavevectors are related through $k_z(p_z) = \sqrt{p_z^2 - 2m(V(\infty) - V(-\infty))/\hbar^2}$. The states $|p_z, \mathcal{L}\rangle$ and $|k_z(p_z), \mathcal{R}\rangle$ are orthogonal

$$\langle p_z', \mathcal{L}|k_z(p_z), \mathcal{R}\rangle = 0, \quad \forall\ p_z', p_z. \tag{S6}$$

The relations between the box and continuum normalizations[S4] of these states for $\epsilon_z > E_V$ are given by

$$\langle p_z', \mathcal{L}|p_z, \mathcal{L}\rangle = \delta_{p_z', p_z} = \frac{2\pi}{L_z}\delta(p_z' - p_z), \tag{S7}$$

$$\begin{aligned}\langle k_z(p_z'), \mathcal{R}|k_z(p_z), \mathcal{R}\rangle &= \delta_{k_z', k_z} = \frac{2\pi}{L_z}\delta(k_z(p_z') - k_z(p_z)) \\ &= \frac{2\pi}{L_z}\left(\frac{\partial k_z(p_z)}{\partial p_z}\right)^{-1}\delta(p_z' - p_z) \\ &= \frac{2\pi}{L_z}\frac{k_z(p_z)}{p_z}\delta(p_z' - p_z).\end{aligned} \tag{S8}$$

With normalizations (S7) and (S8) the moduli of the currents associated with the outgoing waves propagating in the negative and positive $z$-directions are respectively given by

$$j_{\mathcal{L}} = \frac{\hbar p_z}{m L_z}, \qquad j_{\mathcal{R}} = \frac{\hbar k_z}{m L_z}. \tag{S9}$$

and have effective dimension of inverse time. The above normalizations are consistent with treating the photoexcited electron scattering by plasmons in the $z$-direction within the scattering boundary conditions and in the $(x, y)$-direction within the decaying states boundary conditions. Therefore, the division by (S9) is equivalent to multiplication by the duration of the interaction along the $z$-coordinate. This is particularly appropriate to description of electron yield from slab geometries.

The distinction of electronic states with $\epsilon_z < E_V$ and $\epsilon_z > E_V$ is prerequisite to establishing a consistent completeness relation for the states diagonalizing $H_0^{el}$. It reads

$$\begin{aligned}\mathbf{1} &= \sum_{p_z(\epsilon_z < E_V)} |p_z\rangle\langle p_z| + \sum_{p_z(\epsilon_z > E_V)} |p_z, \mathcal{L}\rangle\langle p_z, \mathcal{L}| \\ &+ \sum_{k_z(\epsilon_z > E_V)} |k_z(p_z), \mathcal{R}\rangle\langle k_z(p_z), \mathcal{R}|.\end{aligned} \tag{S10}$$

Using this we can identify the various channels of inelastic electron transitions in plasmon emission or absorption processes. In the situation *(i)* discussed above with both the initial $\epsilon_z < E_V$ and final $\epsilon_z' < E_V$ there is only one scattering channel $|p_z\rangle \to |p_z'\rangle$ with $p_z'$ given by (S5). The next possibility pertains to

$$\epsilon_z = \frac{\hbar^2 p_z^2}{2m} + V(-\infty) = \frac{\hbar^2 k_z^2}{2m} + V(\infty) > E_V \tag{S11}$$

in the initial degenerate electron state, and

$$\epsilon_z' = \frac{\hbar^2 p_z'^2}{2m} + V(-\infty) < E_V \tag{S12}$$

in the final nondegenerate stationary state. In this situation we can distinguish two subsets of electron scattering channels

$$|k_z, \mathcal{R}\rangle \to |p_z'\rangle, \quad |p_z, \mathcal{L}\rangle \to |p_z'\rangle. \tag{S13}$$

Here the final $p_z'$ is given either by expression identical to (S5) or by

$$p_z' = \sqrt{2m(\epsilon_{\mathbf{K}} - \epsilon_{\bar{\mathbf{K}}} + \hbar^2 k_z^2/2m + V(\infty) - V(-\infty) \mp \hbar\omega_{\mathbf{q}})}/\hbar. \tag{S14}$$

*(iii)* Lastly, if the final state is also degenerate, viz.

$$\epsilon_z' = \frac{\hbar^2 p_z'^2}{2m} + V(-\infty) = \frac{\hbar^2 k_z'^2}{2m} + V(\infty) > E_V \tag{S15}$$

we have four distinct subsets of electron-plasmon scattering channels between the initial and final electron states

$$\begin{aligned}&|k_z, \mathcal{R}\rangle \to |k_z', \mathcal{R}\rangle, \quad |k_z, \mathcal{R}\rangle \to |p_z', \mathcal{L}\rangle, \\ &|p_z, \mathcal{L}\rangle \to |p_z', \mathcal{L}\rangle, \quad |p_z, \mathcal{L}\rangle \to |k_z', \mathcal{R}\rangle.\end{aligned} \tag{S16}$$

Using the above introduced enumerations the first step in the regularization of the $\delta$-function in (S1) is to isolate in its argument the values of $k_z'^2/2m$ or $p_z'^2/2m$ and express them in terms of unperturbed $k_z$ and $p_z$ using the above relations (S11) and (S15) as appropriate to a particular scattering channel in (S16). This gives for the scattered or final wavevectors in the specified four sets of channels

$$\ell_1' = \sqrt{\frac{2m}{\hbar^2}}[\epsilon_{\mathbf{K}} + \frac{\hbar^2 k_z^2}{2m} - \epsilon_{\bar{\mathbf{K}}} \mp \hbar\omega_{\mathbf{q}}]^{1/2}, \tag{S17}$$

$$\begin{aligned}\ell_2' &= \sqrt{\frac{2m}{\hbar^2}}[\epsilon_{\mathbf{K}} + \frac{\hbar^2 k_z^2}{2m} + (V(\infty) - V(-\infty)) \\ &\quad -\epsilon_{\bar{\mathbf{K}}} \mp \hbar\omega_{\mathbf{q}}]^{1/2},\end{aligned} \tag{S18}$$

$$\ell_3' = \sqrt{\frac{2m}{\hbar^2}}[\epsilon_{\mathbf{K}} + \frac{\hbar^2 p_z^2}{2m} - \epsilon_{\bar{\mathbf{K}}} \mp \hbar\omega_{\mathbf{q}}]^{1/2}, \tag{S19}$$

$$\begin{aligned}\ell_4' &= \sqrt{\frac{2m}{\hbar^2}}[\epsilon_{\mathbf{K}} + \frac{\hbar^2 p_z^2}{2m} - (V(\infty) - V(-\infty)) \\ &\quad -\epsilon_{\bar{\mathbf{K}}} \mp \hbar\omega_{\mathbf{q}}]^{1/2},\end{aligned} \tag{S20}$$

Note in passing that the thus defined $\ell'$s may also involve energy differences from interband transitions. The corresponding currents are given by $j_{\ell'} = \hbar\ell'/mL_z$. These expressions, together with the auxiliary relation

$$\delta\left(\frac{(\hbar k_z)^2}{2m} - \frac{(\hbar k_z')^2}{2m}\right) = \frac{m}{\hbar^2 k_z}\delta(k_z - k_z') = \frac{1}{2\pi\hbar j_z}\delta_{k_z',k_z}, \tag{S21}$$

enable to transform the energy conserving $\delta$-function in (S1) in each scattering channel to the form

$$\text{channel } \mathcal{R} \to \mathcal{R}: \quad \text{Eq.}(S1) = \frac{\delta_{k_z',\ell_1'}}{\hbar j_{\ell_1'}}\theta(\ell_1'^2), \tag{S22}$$

$$\text{channel } \mathcal{R} \to \mathcal{L}: \quad \text{Eq.}(S1) = \frac{\delta_{p_z',\ell_2'}}{\hbar j_{\ell_2'}}\theta(\ell_2'^2), \tag{S23}$$

$$\text{channel } \mathcal{L} \to \mathcal{L}: \quad \text{Eq.}(S1) = \frac{\delta_{k_z',\ell_3'}}{\hbar j_{\ell_3'}}\theta(\ell_3'^2), \tag{S24}$$

$$\text{channel } \mathcal{L} \to \mathcal{R}: \quad \text{Eq.}(S1) = \frac{\delta_{p_z',\ell_4'}}{\hbar j_{\ell_4'}}\theta(\ell_4'^2). \tag{S25}$$

where $\theta(x)$ is the step function.

Combining the appropriate (S5)-(S25) in expression (33) we obtain for particular scattering channels

$$\begin{aligned} w^{\ell',\ell,}_{\mathbf{K},\bar{\mathbf{K}},\mathbf{Q}} &= \mid 2\pi V^{\ell',\ell}_{\bar{\mathbf{K}},\mathbf{K},\mathbf{Q}}\delta(\epsilon_{\bar{\mathbf{K}}} + \epsilon_{\ell'} - \epsilon_{\mathbf{K}} - \epsilon_\ell \pm \hbar\omega_{\mathbf{q}}) \mid^2 \\ &= \frac{1}{\hbar^2}\left|\frac{V^{\ell',\ell}_{\bar{\mathbf{K}},\mathbf{K},\mathbf{Q}}}{\sqrt{j_\ell j_{\ell'}}}\right|^2. \end{aligned} \tag{S26}$$

where $\ell$ and $\ell'$ run over the initial and final state wavevectors, respectively, discussed within the items *(i)-(iii)* above. The matrix elements $V^{\ell',\ell}_{\bar{\mathbf{K}},\mathbf{K},\mathbf{Q}}$ are calculated in the box normalization, i.e. bear the factor $1/L_z$ which cancels the same factor from the currents $\sqrt{j_\ell j_{\ell'}}$. The factor $1/L^2$ from (S2) is after integration over the lateral $(x, y)$ coordinate absorbed in the factorizable lateral momentum conservation $\delta_{\bar{\mathbf{K}},\mathbf{K}\mp\mathbf{Q}}$ and hence does not appear in $V^{\ell',\ell}_{\bar{\mathbf{K}},\mathbf{K},\mathbf{Q}}$ any more. All this makes (S26) adimensional probabilities free from the quantization lengths and satisfying the time reversal. Note also that in the case of plasmon emission [upper sign in (S17)-(S20)] the probabilities (S26) are summed over both $\mathcal{R}$ and $\mathcal{L}$ final state scattering channels. On the other hand, in the case of plasmon absorption [lower sign in (S17)-(S20)] giving rise to final electron yield outside the surface, only the final $\mathcal{R}$-channels contribute, as formulated in standard theories of surface photoeffect.[S5,S6]

### B. Decaying states boundary conditions

In the case of polarization-induced plasmon generation in bulk systems extending in all three $(x, y, z)$-directions and described by the Hamiltonian (5) there is no preferential direction for definition of excited electron current(s) associated with the running wave(s) $\langle\mathbf{r}|\mathbf{k}\rangle$ leaving the range of interaction $V^{e-pl}$. Hence the photoexcited electron-plasmon scattering is subject to decaying state boundary conditions. In this context we may retain box normalization in all three directions, viz.

$$\langle\mathbf{k}|\bar{\mathbf{k}}\rangle = \delta_{\mathbf{k},\bar{\mathbf{k}}} = \left(\frac{2\pi}{L}\right)^3\delta(\mathbf{k} - \bar{\mathbf{k}}), \tag{S27}$$

which gives the electron decay rate in the form

$$w^{\mathbf{q}}_{\bar{\mathbf{k}},\mathbf{k}} = \mid 2\pi V^{\mathbf{q}}_{\bar{\mathbf{k}},\mathbf{k}}\delta(\epsilon_{\bar{\mathbf{k}}} - \epsilon_{\mathbf{k}} + \hbar\omega_{\mathbf{q}})(1 - n_{\bar{\mathbf{k}}})\delta_{\bar{\mathbf{k}},\mathbf{k}-\mathbf{q}} \mid^2. \tag{S28}$$

Here the factor $1/L^3$ from (S27) that appears in the calculation of matrix element $V^{\mathbf{q}}_{\bar{\mathbf{k}},\mathbf{k}}$ has been absorbed to produce $\delta_{\bar{\mathbf{k}},\mathbf{k}\mp\mathbf{q}}$ and hence (S28) is free from the quantization length factors $L$. This renders (S28) dimensionless, yet still formally divergent. The divergence arises from the second order perturbative treatment of electron excitation to a stable state $|\mathbf{k}\rangle$ in which it could propagate indefinitely within the system, i.e. over the time interval $L/v_{|\mathbf{k}|}$ where $v_{|\mathbf{k}|} = \hbar|\mathbf{k}|/m$. In reality, however, electron propagation in the excited state is restricted by its lifetime and to account for this the probabilities (S28) should be adequately renormalized. The appropriate procedure[S2] has already been applied to photoemission[S3] and for the $|\mathbf{k}\rangle \to |\bar{\mathbf{k}}\rangle$ decay channel yields

$$w_{\bar{\mathbf{k}},\mathbf{k}} = \sum_{\mathbf{q}} w^{\mathbf{q}}_{\bar{\mathbf{k}},\mathbf{k}} \to \sum_{\mathbf{q}} \frac{|V^{\mathbf{q}}_{\bar{\mathbf{k}},\mathbf{k}}|^2(1 - n_{\bar{k}})\delta_{\bar{\mathbf{k}},\mathbf{k}-\mathbf{q}}}{(\epsilon_{\bar{\mathbf{k}}} - \epsilon_{\mathbf{k}} + \hbar\omega_{\mathbf{q}})^2 + (\Gamma_{\mathbf{k}}/2)^2}, \tag{S29}$$

where $\Gamma_{\mathbf{k}}$ is given by (35). Note that likewise in Appendix A, $\mathbf{k}$ and $\bar{\mathbf{k}}$ may also denote different bands. Qualitative illustration of temporal evolution of the various dimensionless transition probabilities towards respective saturation values (S29) corresponding to quasiparticles excited in copper surface bands are presented in Fig. 1 of Ref. [S3].

## S2. FIRST-PRINCIPLES CALCULATIONS OF THE ELECTRONIC STRUCTURE

### A. Ground state

Calculations of the ground-state electronic properties of silver were carried out using the QUANTUM ESPRESSO (QE) code[S7] with a plane-wave cutoff energy of 80 Ry. Optimized norm-conserving Vanderbilt pseudopotentials were used with the PBE exchange-correlation functional.[S8,S9] In order to correctly describe the energy positions of the $d$ bands, the Hubbard on-site interaction $U = 3.1$ eV was implemented and spin-orbit coupling was introduced in order to obtain the band structure along the high-symmetry points [Fig. 7(a) of the main text]. However, it was excluded from later calculations since

the spin-orbit interaction is not crucial for obtaning the correct dielectric function and plasmon energy of bulk silver. A $20 \times 20 \times 20$ Monkhorst-Pack grid was utilized for sampling the *fcc* Brillouin zone (BZ), with Gaussian smearing of 0.01 Ry. The *fcc* unit cell of $a = 4.06$ Åwas used.

### B. Dielectric function

The obtained ground state properties of silver (i.e., electron energies and the corresponding wavefunctions) were utilized in the calculations of the electronic excitation spectra within the random-phase approximation (RPA)[S10,S11]. The dielectric function in the RPA is given by

$$\varepsilon_{\mathbf{G}\mathbf{G}'}(\mathbf{q},\omega) = \delta_{\mathbf{G}\mathbf{G}'} - \sum_{\mathbf{G}_1} v_{\mathbf{G}\mathbf{G}_1}(\mathbf{q})\chi^0_{\mathbf{G}_1\mathbf{G}'}(\mathbf{q},\omega), \tag{S30}$$

where the charge-charge correlation function is given by

$$\chi^0_{\mathbf{G}\mathbf{G}'}(\mathbf{q},\omega) = \frac{2}{\Omega}\sum_{\mathbf{k},nm} \frac{f_{n\mathbf{k}} - f_{m\mathbf{k}+\mathbf{q}}}{\hbar\omega + i\eta + \epsilon_{n\mathbf{k}} - \epsilon_{m\mathbf{k}+\mathbf{q}}} \times M_{n\mathbf{k},m\mathbf{k}+\mathbf{q}}(\mathbf{G})\ M^*_{n\mathbf{k},m\mathbf{k}+\mathbf{q}}(\mathbf{G}'). \tag{S31}$$

Here $n$ and $\mathbf{k}$ denote the band index and wavevector of the bulk electronic state $|n,\mathbf{k}\rangle$, respectively, $\mathbf{G}$ is the reciprocal lattice wavevcector, $v_{\mathbf{G}\mathbf{G}'} = 4\pi/|\mathbf{q}+\mathbf{G}|^2\delta_{\mathbf{G}\mathbf{G}'}$ is the bare Coulomb interaction, $\Omega$ is the normalization volume and $f_{n\mathbf{k}}$ is the Fermi-Dirac distribution function. In these summations we use $120 \times 120 \times 120$ k-mesh sampling and up to 30 electronic bands. For the broadening parameter $\eta$ we use 40 meV. The charge matrix elements are defined as

$$M_{n\mathbf{k},m\mathbf{k}+\mathbf{q}}(\mathbf{G}) = \left\langle \psi_{n\mathbf{k}} \left| e^{-i(\mathbf{q}+\mathbf{G})\mathbf{r}} \right| \psi_{m\mathbf{k}+\mathbf{q}} \right\rangle_V, \tag{S32}$$

where $\mathbf{q}$ is the momentum transfer and $\mathbf{G}$ are the reciprocal lattice vectors. $\psi_{n\mathbf{k}}(\mathbf{r})$ and $\epsilon_{n\mathbf{k}}$ are Kohn-Sham wavefunctions and energies, respectively. The electron energy loss spectrum is obtained by calculating

$$\mathrm{EELS} = -\mathrm{Im}\left[\varepsilon^{-1}_{\mathbf{G}\mathbf{G}'}(\mathbf{q},\omega)\right]_{\mathbf{G}=\mathbf{G}'=\mathbf{0}}, \tag{S33}$$

which then contains plasmon poles as well as the screened interband and intraband excitations.

### C. Electron-plasmon coupling

The electron-plasmon matrix elemets as used in the main text to describe interactions in bulk systems are defined as[S12,S13]

$$V^{\mathrm{e-p}}_{n,\mathbf{k},m\mathbf{q}} = \left[\frac{1}{v(\mathbf{q})}\frac{\partial\varepsilon(\mathbf{q},\omega)}{\partial\omega}\bigg|_{\omega_\mathbf{q}}\right]^{-1/2} M_{n\mathbf{k},m\mathbf{k}+\mathbf{q}}(0), \tag{S34}$$

where $\omega_\mathbf{q}$ are the plasmon frequencies obtained from the poles of the dielectric function, i.e., $\varepsilon(\mathbf{q},\omega_\mathbf{q}) = 0$. In order to simplify the evaluation of Eq. (S34), the dielectric function in the rectangular brackets is approximated as in the homogeneous electron gas, i.e., $\varepsilon(\mathbf{q},\omega) = 1 - \omega^2_\mathbf{q}/\omega^2$. In that case, the electron-plasmon matrix elements are

$$V^{\mathrm{e-p}}_{n\mathbf{k},m\mathbf{q}} = \left[\frac{v(\mathbf{q})\omega_\mathbf{q}}{2}\right]^{1/2} M_{n\mathbf{k},m\mathbf{k}+\mathbf{q}}(0). \tag{S35}$$

Quite generally, in homogeneous systems plasmons are well-defined mode in momentum-frequency space only outside the intraband and interband continua where they are not affected by the Landau damping (i.e., decay into to electron-hole pairs). By examining the electron energy loss spectrum Eq. (S33) in bulk Ag we find that the corresponding plasmon critical wavevector is $q_{\mathrm{cut}} \approx 0.15$ a.u. (yielding $\omega \approx 4.1$ eV), above which the plasmon dispersion curve enters the Landau-damping region. The experimental value of this wavevector is $q^{\mathrm{exp}}_{\mathrm{cut}} \approx 0.1$ a.u. Therefore, all the plasmon momentum integrations appearing in Eqs. (43)-(50) should be performed up to this cut-off value.

Numerical evaluation of the plasmon emission and absorption rates from the main text [i.e., Eqs. (43)-(50)] are performed by means of a modified version of the EPW code[S14], in which the electron-plasmon self-energy utilizing Eq. (S35) is implemented[S13,S15]. For this purpose, the corresponding input quantities (electron energies and electron-plasmon matrix elements) were interpolated using maximally localized Wannier functions[S16] from the recently developed automated wannierization procedure[S17]. Expression (S35) as well as the plasmon emission and absorption rates were calculated on the $30 \times 30 \times 30$ electron $\mathbf{k}$ and plasmon $\mathbf{q}$ wavevector grids. For the corresponding surface calculations the equivalent $30 \times 30 \times 1$ grids were used. We used $q^{\mathrm{exp}}_{\mathrm{cut}} \approx 0.1$ a.u. for the plasmon momentum cut-off and $\omega_\mathbf{q}$ determined numerically from Eq. (S33).

### D. GW correlation self-energy

Correlation self-energy of a Bloch state $|n,\mathbf{k}\rangle$ consists of two terms[S18,S19]

$$\Sigma^C_{n\mathbf{k}}(\mathbf{q},\omega) = \Sigma^{iF}_{n\mathbf{k}}(\mathbf{q},\omega) + \Sigma^{cH}_{n\mathbf{k}}(\mathbf{q},\omega), \tag{S36}$$

where the first term represents the induced Fock self-energy

$$\Sigma^{iF}_{n\mathbf{k}}(\omega) = -\sum_m \int \frac{d\mathbf{q}}{(2\pi)^3} f_{m\mathbf{k}+\mathbf{q}} \times |M_{n\mathbf{k},m\mathbf{k}+\mathbf{q}}|^2\ W^{ind}(\mathbf{q},\omega - \epsilon_{m\mathbf{k}+\mathbf{q}}). \tag{S37}$$

The second term represents the Coulomb-hole contribution

$$\Sigma^{cH}_{n\mathbf{k}}(\omega) = \sum_m \int_{\mathbf{q}\in B.Z} \frac{d\mathbf{q}}{(2\pi)^3} \times \tag{S38}$$

$$|M_{n\mathbf{k},m\mathbf{k+q}}|^2\,\Gamma(\mathbf{q},\omega-\epsilon_{m\mathbf{k+q}}),\text{(S39)}$$

where the correlation propagator is defined as

$$\Gamma(\mathbf{q},\omega)=\int_0^\infty d\omega'\frac{D(\mathbf{q},\omega')}{\omega-\omega'+i\eta},\qquad\text{(S40)}$$

and the spectrum of electronic excitations is defined as

$$D(\mathbf{q},\omega)=-\frac{1}{\pi}\mathrm{Im}\,W^{ind}(\mathbf{q},\omega).$$

The induced part of dinamically screened Colulomb interaction is

$$W^{ind}(\mathbf{q},\omega)=W(\mathbf{q},\omega)-v_{\mathbf{q}},$$

where the bare Coulomb interaction is $v_{\mathbf{q}}=4\pi/q^2$. Then the total, dinamically screened Coulomb interaction reads

$$W(\mathbf{q},\omega)=v_{\mathbf{q}}/\varepsilon(\mathbf{q},\omega).\qquad\text{(S41)}$$

Here the RPA dielectric function is defined as

$$\varepsilon(\mathbf{q},\omega)=1-v_{\mathbf{q}}\chi^0(\mathbf{q},\omega),\qquad\text{(S42)}$$

with the time-ordered RPA response function

$$\chi^0(\mathbf{q},\omega)=\frac{2}{\Omega}\sum_{\mathbf{k},nm}|M_{n\mathbf{k},m\mathbf{k+q}}|^2\times\frac{f_{n\mathbf{k}}-f_{m\mathbf{k+q}}}{\omega+\epsilon_{n\mathbf{k}}-\epsilon_{m\mathbf{k+q}}+i\eta\mathrm{sgn}(\epsilon_{\mathrm{m}\mathbf{k+q}}-\epsilon_{\mathrm{n}\mathbf{k}})}.\qquad\text{(S43)}$$

The $\mathbf{q}$-points mesh used in the integrations over the BZ is $81\times81\times81$. The crystal local field effects are not included. The calculated imaginary part of the electron correlation self-energy [i.e. $\Gamma=-2\mathrm{Im}\Sigma^C_{n\mathbf{k}}(\mathbf{q},\omega)$] for the bulk silver is shown in Fig. 8(b) of the main text. The results are obtained for $\mathbf{k}$ corresponding to the L point in the BZ and for the upper *sp* band centered around 3.8 eV. These results include both the plasmon emission processes as well as electron (intraband and interband) excitations.

### E. Simulations of the Ag(110) surface

Along with the calculations of the various plasmon-induced electron transition rates in bulk Ag we have also performed equivalent calculations for the Ag(110) surface (see Figs. 10, 11, and 12 of the main text). To this end we have made use of the bulk electronic band structure to project it on the (110) plane of the *fcc* Brillouin zone with the $k_z$ momentum conservation along this direction relaxed. Thereby one obtains accurate description of the bulk-projected bands along the Ag(110) surface by using only the results of bulk ground state calculations. However, using this method one neglects the appearance of surface states along Ag(110) because the vacuum side is missing. Although we believe that both the bulk and surface states are important for understanding plasmonic photoemission from Ag, due to computational difficulties encounterred in simulations of real Ag(110) surface, we defer the investigations the effects of surface states to future work.

Comparison of the bulk-projected band structure calculated from bulk Ag bands and the full band structure of Ag(110) obtained for a 51-layer thick slab in the supercell aproach is presented in Fig. S1. It is clear from this figure that all the features of the Ag(110) band structure are well reproduced when the former method is used, the only exception being the surface states.

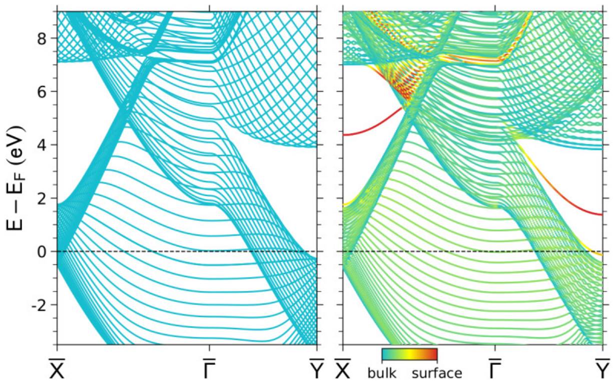


FIG. S1: Left panel: (110) surface-projected band structure of bulk Ag bands. The surface projected continuua are obtained by relaxing the momentum conservation in the direction of the normal to (110) crystal plane. Right panel: The Ag(110) band structure as obtained from the 51-layer slab calculations. The slabs in the adjacent supercells are separated by vacuum. Note the differentiation between bulk and surface character of the various bands as quantified by the color bar.

### F. Averaged plasmon emission and absorption rates

As we are primarily interested in the observed plasmonically assisted photoemission,[S20] we have singled out in Figs. 10, 11, and 12 of the main text only the contributions of the one- and two-plasmon-assisted yields at $\simeq E_F+\hbar\omega_p$ and $\simeq E_F+2\hbar\omega_p$. Thus, in Fig. 10(c) we extract the plasmon absorption rate at $\simeq E_F+\hbar\omega_p$ by defining the isoenergetic distribution of $\gamma^{\mathrm{CFS}(\hbar\omega_p)}_{\mathbf{k}'}$ averaged around $\epsilon_{\mathbf{k}'}\simeq E_F+\hbar\omega_p$ by using the following procedure

$$\left\langle\gamma^{\mathrm{CFS}(\hbar\omega_p)}_{\mathbf{k}'}\right\rangle_{\omega_p}=\frac{\sum_n\gamma^{\mathrm{CFS}(\hbar\omega_p)}_{n\mathbf{k}'}\delta(\epsilon_{n\mathbf{k}'}-E_F-\hbar\omega_p)}{\sum_n\delta(\epsilon_{n\mathbf{k}'}-E_F-\hbar\omega_p)}.\qquad\text{(S44)}$$

Here we use a Gaussian with FWHM of 0.2 eV to approximate the delta functions $\delta(x)$. In the main text the notation $\mathbf{k}'$ actually stands for $n\mathbf{k}'$. Note also that by using this method we only average over the enegies, while retaining the momentum resolution.

To calculate the two-plasmon absorption rates presented in Fig. 11 of the main text, we use Eqs. (49) and (50) where initial state energies $\epsilon_{\mathbf{k}'}$ are taken from the isoenergetic distribution Eq. (S44) at $E_F + \hbar\omega_p$ as shown in Fig. 10(c). The averaging of the isoenergetic distribution presented in Fig. 11(c) is performed likewise in Eq. (S44), i.e.,

$$\left\langle \gamma_{\mathbf{k}''}^{\mathrm{CFS}(2\hbar\omega_p)} \right\rangle_{2\omega_p} = \frac{\sum_n \gamma_{n\mathbf{k}''}^{\mathrm{CFS}(2\hbar\omega_p)} \delta(\epsilon_{n\mathbf{k}''} - E_F - 2\hbar\omega_p)}{\sum_n \delta(\epsilon_{n\mathbf{k}''} - E_F - 2\hbar\omega_p)}, \tag{S45}$$

with the same approximation for the delta-functions.

In calculating the resonant rate $\gamma_{\mathbf{k}''}^{\mathrm{res}(2\hbar\omega_p)}$ we again take into account only the processes making up the following sequence $\epsilon_{\mathbf{k}} \simeq E_F \to \epsilon_{\mathbf{k}'} \simeq E_F + \hbar\omega_p \to \epsilon_{\mathbf{k}''} \simeq E_F + 2\hbar\omega_p$. Therefore, we evaluate expression (50) as

$$\gamma_{\mathbf{k}''}^{\mathrm{res}(2\hbar\omega_p)} \simeq \frac{\pi}{2}\rho_f(\epsilon_{\mathbf{k}''}) \sum_{\mathbf{k}'} \gamma_{\mathbf{k}'',\mathbf{k}'}^{(2\hbar\omega_p)} \left\langle \gamma_{\mathbf{k}'}^{\mathrm{CFS}(\hbar\omega_p)} \right\rangle_{\omega_p}. \tag{S46}$$

Finally, the isoenergetic distribution of Eq. (50) averaged around $\epsilon_{\mathbf{k}''} \simeq E_F + 2\hbar\omega_p$ and shown in Fig. 12 is obtained as

$$\left\langle \gamma_{\mathbf{k}''}^{\mathrm{res}(2\hbar\omega_p)} \right\rangle_{2\omega_p} = \frac{\sum_n \gamma_{n\mathbf{k}''}^{\mathrm{res}(2\hbar\omega_p)} \delta(\epsilon_{n\mathbf{k}''} - E_F - 2\hbar\omega_p)}{\sum_n \delta(\epsilon_{n\mathbf{k}''} - E_F - 2\hbar\omega_p)}. \tag{S47}$$


[S1] B. Gumhalter, Phys. Rep. **351**, 1 (2001).
[S2] I. Adawi, Phys. Rev. **134**, A788 (1964).
[S3] Simple one-dimensional examples of such orthogonal states are the functions $u^*(z)$ and $v^*(z)$ discussed in Sec. II.B. of Ref. [S5].
[S4] E.E. Krasovskii, V.M. Silkin, V.U. Nazarov, P.M. Echenique, and E.V. Chulkov, Phys. Rev. B **82**, 125102 (2010).
[S5] A. Messiah, *Quantum Mechanics*, Vol.II, North Holland, Amsterdam 1965, Ch. XXI/13.
[S6] F. El Shaer and B. Gumhalter, Phys. Rev. Lett. **93**, 236804, (2004)).
[S7] P. Giannozzi, S. Baroni, N. Bonini *et al.*, J Phys.: Condens. Matter **21**, 395502 (2009).
[S8] D. R. Hamann, Phys. Rev. B 88, 085117
[S9] J. P. Perdew, K. Burke, and M. Ernzerhof, Phys. Rev. Lett.**77**, 3865 (1996).
[S10] V. Despoja, D. Novko, K. Dekanić, M. Šunjić, and L. Marušić, Phys. Rev. B **87**, 075447 (2013).
[S11] D. Novko, V. Despoja, and M. Šunjić, Phys. Rev. B **91**, 195407 (2015).
[S12] D. Pines and J. R. Schrieffer, Phys. Rev. **125**, 804, 1962.
[S13] F. Caruso and F. Giustino, Phys. Rev. B **94**, 115208 (2016).
[S14] S. Poncé, E. Margine, C. Verdi, and F. Giustino, Comput. Phys. Commun. **209**, 116 (2016).
[S15] F. Caruso, C. Verdi, S. Poncé, and F. Giustino, Phys. Rev. B **97**, 165113 (2018).
[S16] N. Marzari, A. A. Mostofi, J. R. Yates, I. Souza, and D.Vanderbilt, Rev. Mod. Phys. **84**, 1419 (2012).
[S17] V. Vitale, G. Pizzi, A. Marrazzo, J. R. Yates, N. Marzari, A. A. Mostofi, npj Comput. Mater. **6**, 66 (2020).
[S18] M. Rohlfing and S. G. Louie Phys. Rev. B **62**, 4927 (2000).
[S19] Z. Rukelj, V. Despoja, New J. Phys. **22**, 063052 (2020).
[S20] A. Li, M. Reutzel, Z. Wang, D. Novko, B. Gumhalter, and H. Petek, ACS Photonics **8**, 1, 247 (2021).
